# Supplementary material for: Benchmark Dataset Dynamics, Bias and Privacy Challenges in Voice Biometrics Research
Source: arXiv:2304.03858 source file (2023-08-18)
Supplement: Supplementary file 1 [file appendix.tex]

\newpage
\section{Appendix}
\label{appendix}

\subsection{Supplementary Figures for Section~\ref{s:method} - Research Approach}

\begin{figure}[hbt]
    \centering
    \includegraphics[width=0.4\linewidth]{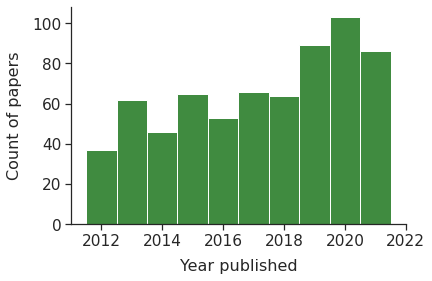}
    \caption{Histogram of papers published at Interspeech over the past decade and analyzed in this study.}
    \label{fig:interspeech_paper_count}
\end{figure}

\subsection{Supplementary Figures for Section~\ref{ss:dataset_adoption} - Community Adoption of Speaker Recognition Datasets}

\begin{figure}[hbt]
    \centering
    \includegraphics[width=\textwidth]{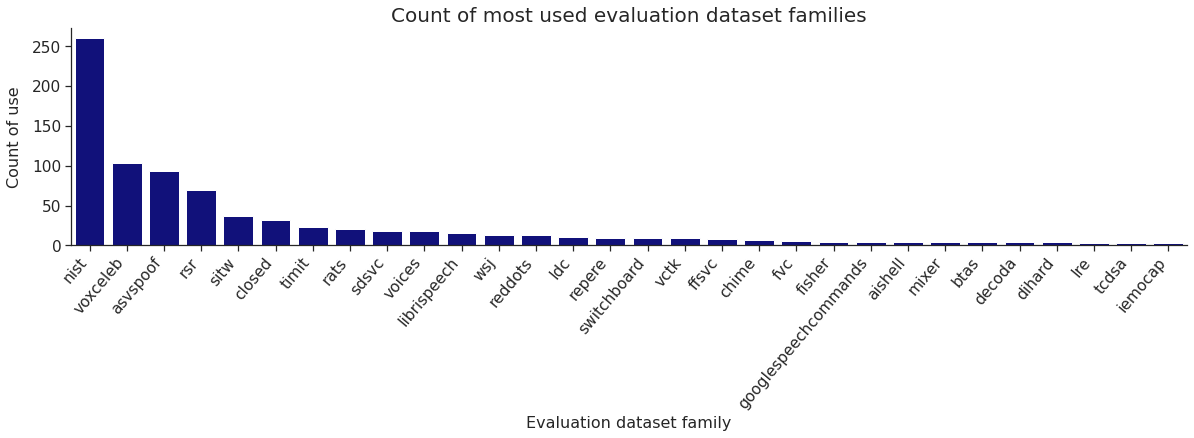}
    \caption{Histogram showing the count of most used evaluation dataset families between 2012 and 2021.}
\label{fig:eval_frequency}
\end{figure}

\clearpage
\subsection{Supplementary Figures for Section~\ref{ss:datasetattributes} - Dataset Attributes}

\begin{figure}[hbt]
    \centering
    \includegraphics[width=0.95\textwidth]{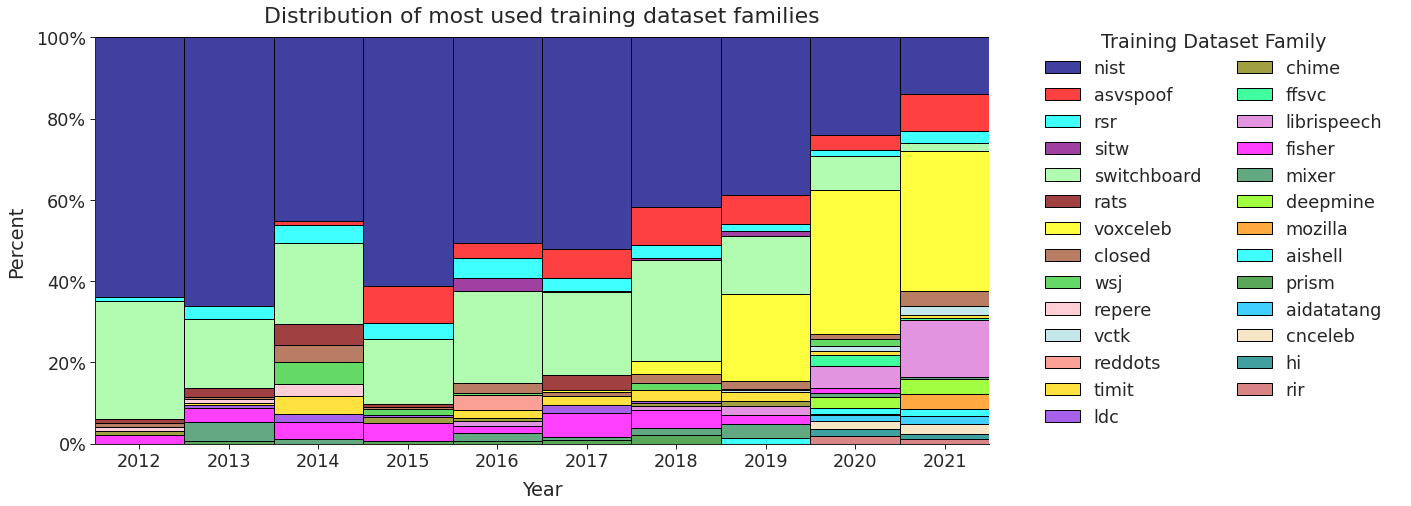}
    \caption{Distribution (\%) of \textbf{dataset family} use for speaker recognition \textbf{training}.}
\label{fig:train_family_density}
\end{figure}

\begin{figure}[hbt]
    \centering
    \includegraphics[width=0.95\textwidth]{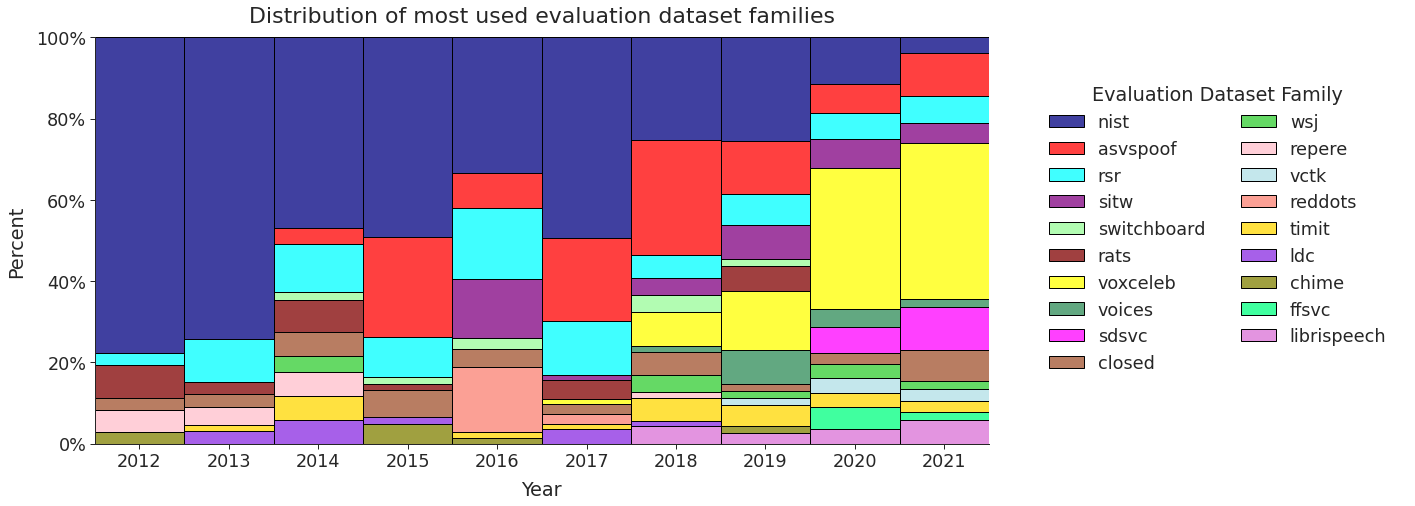}
    \caption{Distribution (\%) of \textbf{dataset family} use for speaker recognition \textbf{evaluation}.}
\label{fig:eval_family_density}
\end{figure}

\begin{table}[hbt]
\begin{tabular}{c|cccc}
\textbf{Year} & \thead{Published\\papers} & \thead{1 evaluation dataset\\only} & \thead{1 VoxCeleb dataset\\only} & \thead{VoxCeleb1 - test\\only} \\ \midrule
\textbf{2012} & 37 & 26 (70\%) & - & - \\
\textbf{2013} & 62 & 46 (74\%) & - & - \\
\textbf{2014} & 46 & 33 (72\%) & - & - \\
\textbf{2015} & 65 & 55 (85\%) & - & - \\
\textbf{2016} & 53 & 39 (74\%) & - & - \\
\textbf{2017} & 66 & 47 (71\%) & 1 & - \\
\textbf{2018} & 64 & 40 (63\%) & 4 (6\%) & 2 (3\%) \\
\textbf{2019} & 89 & 59 (66\%) & 15 (17\%) & 11 (12\%) \\
\textbf{2020} & 103 & 75 (73\%) & 22 (21\%) & 13 (13\%)  \\
\textbf{2021} & 86 & 55 (64\%) & 10 (12\%) & 7 (8\%)  \\
\end{tabular}
\caption{Most speaker recognition studies evaluate their models on a single dataset. A large number of studies evaluate on only one dataset from the VoxCeleb family, or even only on VoxCeleb1 - test.}
\label{tab:eval_with_voxceleb}
\end{table}

\clearpage

\begin{table}[htb]
\small
\resizebox{\linewidth}{!}{
\begin{tabular}{L{0.15\linewidth}|L{0.35\linewidth}|L{0.08\linewidth}|L{0.3\linewidth}|}
%\caption{Overview of development and evaluation data provided by the NIST Speaker Recognition Evaluation (SRE). Each development and evaluation dataset is further divided into training and test data. Our analysis shows the corpora that have been used for development and evaluation.}
%\label{tab:NISTOverview}\\
\textbf{Name and Year} & \textbf{Development Data} & \textbf{Add. Dev. Data} & \textbf{Test Data} \\ \midrule
1996 SR Benchmark & SWB-1 & \xmark & SWB-1  \\
1997 SR Benchmark & 1996 Development \& Evaluation Data & \xmark & SWB-2 Phase-1  \\
1998 SR Benchmark & 1997 Evaluation Data & \xmark & SWB-2 Phase-2 \\
1999 SR Benchmark & 1998 Evaluation Data & \xmark & SWB-2 Phase-3 \\
2000 NIST SRE & 1999 Evaluation Data \& Callhome Corpus \& SWB-1 & \xmark & SWB-2 Phases 1 \& 2 \& AHUMADA Corpus \& Callhome Corpus  \\
2001 NIST SRE & 2000 Development Data \& SWB-2 Phase 4 \& SWB-1 & \xmark & 2000 Evaluation Data \& SWB-2 Phase 4 \& SWB-1  \\
2002 NIST SRE & 2001 Evaluation Data \& FBI Voice Dataset & \xmark & SWB Cellular Corpus Part 2, SWB-2 Phases 2 \& 3 \& SWB \& CallHome and CallFriend Corpora \\
2003 NIST SRE & 2002 Evaluation Data & \xmark & SWB Cellular Part 2, SWB-2 Phases 2 \& 3 \\
2004 NIST SRE & 2003 Evaluation Data \& SWB-1 & \checkmark & Mixer \\
2005 NIST SRE & 2004 Evaluation Data \& SWB-1  & \checkmark & Mixer  \\ 
2006 NIST SRE & 2004 Evaluation Data \& 2005 Evaluation Data \& SWB-1 & \checkmark & Mixer 1, 2 \& 3  \\ 
2008 NIST SRE & All previous NIST SRE evaluation data \& interview speech & \checkmark & Mixer 5 \\ 
2010 NIST SRE & All previous NIST SRE evaluation data \& high/low vocal effort speech & \checkmark & Mixer 6 \\
2012 NIST SRE & All previous NIST SRE data & \checkmark & n.a. \\
2016 NIST SRE & Fixed training condition: Call My Net Corpus \& all previous NIST SRE data \& SWB corpora \& Fisher corpus & (\checkmark) & Call My Net \\
2018 NIST SRE & Fixed training condition: 1996–2008 NIST SRE Data \& 2010 NIST SRE \& Follow-up Data \&  2012 NIST SRE Test Set \& 2016 NIST SRE Development \& Test Set \& Comprehensive SWB \& Comprehensive Fisher English \& Mixer 6 \& 2018 NIST SRE Development Set & (\checkmark) & Call My Net 2 \& Video Annotation for Speech \\  
2019 NIST SRE & & (\checkmark) & Call My Net 2 \& Video Annotation for Speech Technology \\
2021 NIST SRE & Fixed training condition: NIST SRE CTS Superset \& 2016 NIST SRE EValuation Set \& 2021 NIST SRE Development Set \& JANUS Multimedia Dataset \& VoxCeleb & (\checkmark) & WeCanTalk corpus \\
%\end{longtable}}
\end{tabular}}
\caption{Overview of development and evaluation data provided by the NIST Speaker Recognition Evaluation (SRE). We display whether participating sites were allowed to use additional data for development (\xmark: no additional data was allowed, \checkmark: additional data allowed, (\checkmark): additional data allowed in the open condition).}
\label{tab:NISTOverview}
\end{table}

\noindent \textbf{Abbreviations} \\
LDC: Linguistic Data Consortium in consultation with Lincoln Laboratory\\
NIST: National Institute for Standards and Technology\\
SID: Speaker Identification research community\\
FBI: United States Federal Bureau of Investigation\\
DOD: United States Department of Defense\\
ITIC: Intelligence Technology Innovation Center\\

\begin{landscape}
\begin{table}
\scriptsize

\begin{longtable}{L{0.07\linewidth}|L{0.1\linewidth}|L{0.1\linewidth}|L{0.11\linewidth}|L{0.11\linewidth}|L{0.1\linewidth}|L{0.11\linewidth}|L{0.11\linewidth}}
\textbf{Shorthand} & \textbf{-} & \textbf{SWB-1} & \textbf{SWB-2 Phase I} & \textbf{SWB-2 Phase II} & \textbf{SWB-2 Phase III} & \textbf{-} & \textbf{-} \\
\textbf{Dataset name} & \textbf{Switchboard Credit Card} ~\cite{Godfrey1993SwitchboardCC} & \textbf{Switchboard-1 Release 2}~\cite{Godfrey1997Switchboard1} & \textbf{Switchboard-2 Phase I}~\cite{Graff1998Switchboard2I} & \textbf{Switchboard-2 Phase II}~\cite{Graff1999Switchboard2II} & \textbf{Switchboard-2 Phase III Audio}~\cite{Graff2002Switchboard2III} & \textbf{Switchboard Cellular Part 1 Audio}~\cite{Graff2001SwitchboardCellularPart1} & \textbf{Switchboard Cellular Part 2 Audio}~\cite{Graff2004SwitchboardCellularPart2} \\ \midrule
\textbf{Authors} & John J. Godfrey, Ed Holliman & John J. Godfrey, Edward Holliman & David Graff, Alexandra Canavan, George Zipperlen & David Graff, Kevin Walker, Alexandra Canavan & David Graff, David Miller, Kevin Walker & David Graff, Kevin Walker, David Miller & David Graff, Kevin Walker, David Miller \\
\textbf{Link} &  \url{https://catalog.ldc.upenn.edu/LDC93S8} & \url{https://catalog.ldc.upenn.edu/LDC97S62} & \url{https://catalog.ldc.upenn.edu/LDC98S75} & \url{https://catalog.ldc.upenn.edu/LDC99S79} & \url{https://catalog.ldc.upenn.edu/LDC2002S06} & \url{https://catalog.ldc.upenn.edu/LDC2001S13} & \url{https://catalog.ldc.upenn.edu/LDC2004S07} \\
\textbf{Collection time frame} & - & 1991-2 & 1996 & 1997 & 1997-8 & 1999-2000 & 2000 \\
\textbf{Collected by} & - & Texas Instruments & LDC & LDC & LDC & LDC & LDC \\
\textbf{Sponsored by} & - & DARPA & DOD & DOD & - & - & - \\
\textbf{Year released} & 1993 & 1992-3 (1997 re-released) & 1998 & 1999 & 2002 & 2001 & 2004 \\
\textbf{Recording device} & - & - & phones with different (ANI) codes & phones with different (ANI) codes & a variety of telephone (land line) handsets & The Switchboard cellular collection focused primarily on GSM cellular phone technology & cellular phone technology of all service types \\
\textbf{Project(s)} & NIST SRE & EARS, GALE, Hub5-LVCSR, NIST SRE & EARS, GALE, NIST SRE, SID & EARS, GALE, NIST SRE, SID & SID, GALE, EARS, NIST SRE & SID, GALE, EARS, NIST SRE & SID, GALE, EARS, NIST SRE \\
\textbf{Application(s)} & speech recognition & speaker identification, speech recognition & speaker identification & speaker identification & speaker identification & speaker identification & speaker identification, language identification \\
\textbf{Total speakers} & 69 & 543 & 657 & 679 & 640 & 254 & 419 \\
\textbf{Total utterances} & 35 two-sided conversations & 2,400 two-sided telephone conversations & 3,638 two-sided 5-minute telephone conversations & 4,472 two-sided five-minute telephone conversations & 2,728 two-sided five-six minute calls & 2,728 two-sided five-six minute calls & 2,020 two-sided five-six minute calls; or 4,040 sides (2,950 cellular) \\
\textbf{Total length} & 227 minutes & 260 hours & na & na & 222 hours & 109 hours & 200 hours \\
\textbf{\# females} & 33 & 241 & 358 & 352 & 348 & 125 & 2405 (samples) \\
\textbf{\# males} & 36 & 302 & 299 & 327 & 292 & 129 & 1635 (samples) \\
\textbf{Manual auditing metadata} & echo, static & echo, static, background data & echo/crosstalk, background noise, distortion & echo/crosstalk, background noise, distortion & echo/crosstalk, background noise, distortion & channel quality, background noise & channel quality, background noise \\
\textbf{Transcribed} & Yes & Yes & No & No & No & No & No \\
\textbf{Speaker attributes (metadata categories)} & sex, year born, dialect area, education level & sex, year born, dialect area, education level & age, sex, years of completed education, country of birth, city and state where raised & age, sex, years of completed education, country of birth, city and state where raised & age, sex, years of completed education, country of birth, city and state where raised & age, sex, years of completed education, country of birth, city and state where raised & age, sex, years of completed education, country of birth, city and state where raised \\
\label{tab:switchboard}
\end{longtable}
\caption{Overview of relevant attributes of the Switchboard datasets.}
\end{table}
\end{landscape}

\begin{landscape}
\begin{table}
\scriptsize

\begin{longtable}{L{0.07\linewidth}|L{0.15\linewidth}|L{0.17\linewidth}|L{0.17\linewidth}|L{0.17\linewidth}|L{0.17\linewidth}}
\textbf{Dataset name} & \textbf{Mixer 1 \cite{CieriMixer1}} & \textbf{Mixer 2} \cite{CieriMixer2} & \textbf{Mixer 3} \cite{CieriMixer3} & \textbf{Mixer 4 and 5}\footnote{\url{https://catalog.ldc.upenn.edu/LDC2020S03}} \cite{CieriMixer3} & \textbf{Mixer 6}\footnote{\url{https://catalog.ldc.upenn.edu/LDC2013S03}} \cite{BrandschainMixer6}\\ \midrule
\textbf{Authors} & Christopher Cieri, Joseph P. Campbell, Hirotaka Nakasone, David Miller,
Kevin Walker & Christopher Cieri, Walt Andrews, Joseph P. Campbell, George Doddington, Jack Godfrey, Shudong Huang, Mark Liberman, Alvin Martin, Hirotaka Nakasone, Mark Przybocki, Kevin Walker & Christopher Cieri, Linda Corson, David Graff, Kevin Walker & Linda Brandschain, Kevin Walker, David Graff, Christopher Cieri, Abby Neely, Nikki Mirghafori, Barbara Peskin, Jack Godfrey, Stephanie Strassel, Fred Goodman, George R. Doddington, Mike King & Linda Brandschain, David Graff, Kevin Walker, Christopher Cieri \\
\textbf{Link} & - & - & - & \url{https://catalog.ldc.upenn.edu/LDC2020S03} & \url{https://catalog.ldc.upenn.edu/LDC2013S03} \\
\textbf{Collection time frame} & 2003 - 2004 & overlapping with Mixer 2 & collected for NIST SRE 2006 & 2007 & 2009 - 2010\\
\textbf{Collected by} & LDC & LDC, Lincoln Laboratory, NIST, SID & LDC & LDC, International Computer Science Institute (ICSI) & LDC \\
\textbf{Sponsored by} & FBI & FBI, DOD, ITIC & - & - & - \\
\textbf{Year released} & - & after 2006 & - & 2020 & 2013 \\
\textbf{Recording device} & a variety of phone handsets and multichannel sensors & a variety of phone handsets and 8 different microphones & a variety of phone handsets & variety of phone handsets and 14 different microphones & a variety of phone handsets, 15 different microphones, two different cell phones \\
\textbf{Data source} & conversational telephone speech & conversational telephone speech & conversational telephone speech & conversational telephone speech and interviews & conversational telephone speech and interviews \\
\textbf{Project(s)} & MIXER, NIST SRE & MIXER, NIST SRE & - & MIXER, NIST SRE & MIXER, NIST SRE\\
\textbf{Application(s)} & speaker recognition & speaker recognition & speaker recognition & speaker identification & speaker identification \\
\textbf{Languages} & Arabic, Mandarin, Russian, Spanish, English & Arabic, Mandarin, Russian, Spanish, English & Bengali, 4 dialects of Chinese, 3 dialects of English, Farsi, Hindi, Italian, Japanese, Korean, Russian, Spanish, Tagalog, Thai, Urdu, and Vietnamese & English & English \\ 
\textbf{Total speakers} & 1402 & - & 3918 & 616 & 594 \\
\textbf{Total utterances} & 15,254
total conversational sides (7627 calls) & - & 19,951 calls & 2,568 recordings made via the public telephone network and 2,152 sessions of multiple microphone recordings in office-room settings & 4,410 recordings made via the public telephone network and 1,425 sessions of multiple microphone recordings in office-room settings \\
\textbf{Total length} & - & - & - & 14,185 hours & 15,863 hours \\
\textbf{\# females} & 58\% female speakers & - & - & - & - \\
\textbf{\# males} & 42\% male speakers & - & -  & - & -\\
\textbf{Manual auditing metadata} & Yes & Yes & - & Yes & -\\
\textbf{Transcribed} & Transcript Reading & Transcript Reading & - & Yes & Transcript Reading \\ 
\textbf{Speaker attributes (metadata categories)} & - & general demographics of speakers & - & sex, year of birth, years of formal education, highest education degree earned, year in which highest degree was earned, educational continuity, age when English was learned, native language, other languages, occupation, place of birth, country where raised, state where raised, city where raised, ethnicity, smoker status, height, weight, mother's place of birth, mother's place of raising, mother's native language, mother's years of formal education, father's place of birth, father's place of raising, father's native language, father's years of formal education & sex, year of birth, years of formal education, highest education degree earned, year in which highest degree was earned, educational continuity, age when English was learned, native language, other languages, occupation, place of birth, country where raised, state where raised, city where raised, ethnicity, smoker status, height, weight, mother's place of birth, mother's place of raising, mother's native language, mother's years of formal education, father's place of birth, father's place of raising, father's native language, father's years of formal education\\
\label{tab:mixer}
\end{longtable}
\caption{Overview of relevant attributes of the Mixer Phases. Information on Phase 2 is limited as it was overlapping with Phase 1.}
\end{table}
\end{landscape}
